# Supplementary material for: Simultaneous Learning of Several Materials Properties from Incomplete Databases with Multi-Task SISSO
Source: arXiv:1901.00948 ancillary file (2019-01-04)
Supplement: Supplementary file 1 [file MT-SISSO_SM.pdf]

# Supplementary Materials

# Simultaneous and Robust Learning of Materials Properties from Heterogeneous and Incomplete Databases with Multi-Task SISSO

Runhai Ouyang,* Emre Ahmetcik, Christian Carbogno,

Matthias Scheffler, and Luca M. Ghiringhelli†

*Fritz-Haber-Institut der Max-Planck-Gesellschaft, 14195 Berlin-Dahlem, Germany*

(Dated: January 3, 2019)

TABLE I: The materials and corresponding primary features for the prototypes $MoS_2$ and $CdI_2$. Atomic features and the materials of other prototypes can be found from the Ref[?] .

| Mater. | prototype | category | $V_{\mathrm{cell}}/\sum V_{\mathrm{atom}}$ | $d_{AB}$ | $CN_A$ | $CN_B$ | $x_A$ | $x_B$ |
|---|---|---|---|---|---|---|---|---|
| $HfTe_2$ | $CdI_2$ | metal | 2.0208 | 2.8222 | 6 | 3 | 0.333 | 0.667 |
| $TiTe_2$ | $CdI_2$ | metal | 2.0438 | 2.7174 | 6 | 3 | 0.333 | 0.667 |
| $CrSe_2$ | $CdI_2$ | metal | 2.3005 | 2.4572 | 6 | 3 | 0.333 | 0.667 |
| $NiTe_2$ | $CdI_2$ | metal | 2.2792 | 2.5928 | 6 | 3 | 0.333 | 0.667 |
| $PdTe_2$ | $CdI_2$ | metal | 2.1756 | 2.6593 | 6 | 3 | 0.333 | 0.667 |
| $PtTe_2$ | $CdI_2$ | metal | 2.2513 | 2.6658 | 6 | 3 | 0.333 | 0.667 |
| $VS_2$ | $CdI_2$ | metal | 2.0903 | 2.3500 | 6 | 3 | 0.333 | 0.667 |
| $VSe_2$ | $CdI_2$ | metal | 2.0200 | 2.4665 | 6 | 3 | 0.333 | 0.667 |
| $CoBr_2$ | $CdI_2$ | nonmetal | 3.1489 | 2.6206 | 6 | 3 | 0.333 | 0.667 |
| $FeBr_2$ | $CdI_2$ | nonmetal | 3.0999 | 2.6536 | 6 | 3 | 0.333 | 0.667 |
| $MnBr_2$ | $CdI_2$ | nonmetal | 3.1589 | 2.7287 | 6 | 3 | 0.333 | 0.667 |
| $VBr_2$ | $CdI_2$ | nonmetal | 2.5777 | 2.6683 | 6 | 3 | 0.333 | 0.667 |
| $VCl_2$ | $CdI_2$ | nonmetal | 2.7425 | 2.5398 | 6 | 3 | 0.333 | 0.667 |
| $CoI_2$ | $CdI_2$ | nonmetal | 2.9248 | 2.8269 | 6 | 3 | 0.333 | 0.667 |
| $FeI_2$ | $CdI_2$ | nonmetal | 2.9840 | 2.8836 | 6 | 3 | 0.333 | 0.667 |
| $HfS_2$ | $CdI_2$ | nonmetal | 2.0806 | 2.5572 | 6 | 3 | 0.333 | 0.667 |
| $HfSe_2$ | $CdI_2$ | nonmetal | 2.0253 | 2.6541 | 6 | 3 | 0.333 | 0.667 |
| $MnI_2$ | $CdI_2$ | nonmetal | 3.0286 | 2.9454 | 6 | 3 | 0.333 | 0.667 |
| $PbI_2$ | $CdI_2$ | nonmetal | 3.5212 | 3.1536 | 6 | 3 | 0.333 | 0.667 |
| $VI_2$ | $CdI_2$ | nonmetal | 2.5694 | 2.8883 | 6 | 3 | 0.333 | 0.667 |
| $PtO_2$ | $CdI_2$ | nonmetal | 2.8082 | 2.0979 | 6 | 3 | 0.333 | 0.667 |
| $PtS_2$ | $CdI_2$ | nonmetal | 2.7072 | 2.4023 | 6 | 3 | 0.333 | 0.667 |
| $PtSe_2$ | $CdI_2$ | nonmetal | 2.4449 | 2.4992 | 6 | 3 | 0.333 | 0.667 |
| $CdI_2$ | $CdI_2$ | nonmetal | 3.0398 | 2.9854 | 6 | 3 | 0.333 | 0.667 |
| $MgBr_2$ | $CdI_2$ | nonmetal | 3.0075 | 2.7014 | 6 | 3 | 0.333 | 0.667 |
| $SnS_2$ | $CdI_2$ | nonmetal | 3.2308 | 2.5672 | 6 | 3 | 0.333 | 0.667 |
| $ZrS_2$ | $CdI_2$ | nonmetal | 2.1032 | 2.5668 | 6 | 3 | 0.333 | 0.667 |

| | | | | | | | | |
|---|---|---|---|---|---|---|---|---|
| $SnSe_2$ | $CdI_2$ | nonmetal | 2.9729 | 2.6741 | 6 | 3 | 0.333 | 0.667 |
| $ZrSe_2$ | $CdI_2$ | nonmetal | 1.8385 | 2.5703 | 6 | 3 | 0.333 | 0.667 |
| $GdI_2$ | $MoS_2$ | metal | 2.0043 | 3.0130 | 6 | 3 | 0.333 | 0.667 |
| $MoS_2$ | $MoS_2$ | nonmetal | 2.1259 | 2.3851 | 6 | 3 | 0.333 | 0.667 |
| $MoSe_2$ | $MoS_2$ | nonmetal | 2.0282 | 2.4907 | 6 | 3 | 0.333 | 0.667 |
| $MoTe_2$ | $MoS_2$ | nonmetal | 2.0072 | 2.6786 | 6 | 3 | 0.333 | 0.667 |
| $WS_2$ | $MoS_2$ | nonmetal | 1.9291 | 2.3855 | 6 | 3 | 0.333 | 0.667 |
| $WSe_2$ | $MoS_2$ | nonmetal | 1.8829 | 2.4973 | 6 | 3 | 0.333 | 0.667 |

TABLE II: The descriptors from leave-prototype-out training (trained on all prototypes except the left out prototype) by using MT-SISSO and global ST-SISSO. The training accuracy for all the MT-SISSO descriptors are 100%. For the global ST-SISSO descriptors, the training accuracy are: 95.65% ($CaF_2$ left-out), 95.41% ($CdI_2$ left-out), 94.29% (CsCl left-out), 92.34% (Mixed left-out), 94.55% (NaCl left-out), 94.46% ($Th_3P_4$ left-out), 93.19% ($TiO_2$ left-out). The generalization test results of the MT-SISSO and global ST-SISSO descriptors on the left out prototypes are shown in Figure 1.

| left-out prototype | MT-SISSO | global ST-SISSO |
|---|---|---|
| CsCl | $d_1 = \frac{V_{\text{cell}}}{\sum V_{\text{atom}}} \frac{IE_A \chi_B \exp(r_{cov,A})}{\chi_A r_{cov,A}}$<br>$d_2 = \frac{V_{\text{cell}}}{\sum V_{\text{atom}}} \frac{IE_A IE_B r_{cov,A} \sqrt{\chi_A}}{\exp(\chi_A)}$ | $d_1 = \left(\frac{\sum V_{\text{atom}}}{V_{\text{cell}}}\right)^2 \frac{\chi_A}{IE_B} \left\| \frac{r_{cov,B}}{r_{cov,A}} - \|x_A - x_B\| \right\|$<br>$d_2 = \frac{\chi_A}{\chi_B} \log(CN_B) + \frac{CN_A}{CN_B} - \frac{d_{AB}}{r_{cov,A}}$ |
| $TiO_2$ | $d_1 = \frac{V_{\text{cell}}}{\sum V_{\text{atom}}} \frac{IE_B r_{cov,A}}{\chi_A} \|IE_A - 2IE_B\|$<br>$d_2 = \frac{V_{\text{cell}}}{\sum V_{\text{atom}}} \frac{IE_A \chi_B}{r_{cov,A}} \exp(r_{cov,A}/\chi_A)$ | $d_1 = \frac{\|x_B - x_A - r_{cov,B}/d_{AB}\|}{(d_{AB} - r_{cov,A}) IE_B / CN_A}$<br>$d_2 = \sqrt{\frac{V_{\text{cell}}}{\sum V_{\text{atom}}} \frac{\chi_B}{\chi_A} (d_{AB} - r_{cov,A}) x_A IE_B}$ |
| $CdI_2$ | $d_1 = \exp\left(\frac{V_{\text{cell}}}{\sum V_{\text{atom}} \chi_A}\right) (IE_A IE_B r_{cov,A})$<br>$d_2 = IE_A d_{AB}^2 \log(IE_B / r_{cov,B})$ | $d_1 = \frac{\sum V_{\text{atom}}}{V_{\text{cell}}} \frac{r_{cov,B}/r_{cov,A} - \|x_A - x_B\|}{IE_B r_{cov,B} x_B}$<br>$d_2 = \frac{V_{\text{cell}}}{\sum V_{\text{atom}}} \frac{(x_A/x_B - x_B^2)\chi_B}{\chi_A CN_B}$ |
| $Th_3P_4$ | $d_1 = \frac{V_{\text{cell}}}{\sum V_{\text{atom}}} IE_A IE_B r_{cov,A}/\chi_A$<br>$d_2 = \frac{V_{\text{cell}}}{\sum V_{\text{atom}}} d_{AB} IE_A \exp(\chi_B)$ | $d_1 = \frac{\sum V_{\text{atom}}}{V_{\text{cell}}} \frac{r_{cov,B}/r_{cov,A} - \|x_A - x_B\|}{IE_B r_{cov,B} x_A}$<br>$d_2 = \frac{IE_B \chi_B}{\chi_A CN_B} \|x_B r_{cov,B} - d_{AB} + r_{cov,A}\|$ |
| $CaF_2$ | $d_1 = \exp\left(\frac{V_{\text{cell}}}{\sum V_{\text{atom}}}\right) \frac{IE_A IE_B r_{cov,A} \chi_B}{\exp(\chi_A)}$<br>$d_2 = \frac{(d_{AB} IE_A)^3}{\chi_B^2} \|IE_A - IE_B\|$ | $d_1 = \frac{\exp(\chi_A) r_{cov,A} CN_A}{\|x_B^3 - x_B + x_A\|}$<br>$d_2 = \frac{V_{\text{cell}}}{\sum V_{\text{atom}}} \frac{IE_B x_A \exp(r_{cov,A}/CN_A)}{\chi_A}$ |
| mixed-prototype | $d_1 = \frac{V_{\text{cell}}}{\sum V_{\text{atom}}} \frac{IE_A IE_B r_{cov,A}}{\chi_A}$<br>$d_2 = IE_A^2 \log(\chi_B) - IE_A IE_B$ | $d_1 = \left(\frac{\sum V_{\text{atom}}}{V_{\text{cell}}}\right)^2 \frac{\chi_A}{IE_B} \left\| \frac{r_{cov,B}}{r_{cov,A}} - \|x_A - x_B\| \right\|$<br>$d_2 = \frac{r_{cov,A}}{x_A d_{AB}} + \frac{\chi_A \log(CN_B)}{\chi_B}$ |
| NaCl | $d_1 = \log(d_{AB} IE_B V_{\text{cell}} / \sum V_{\text{atom}})$<br>$d_2 = \chi_B - \log(\chi_A)$ | $d_1 = \frac{\sqrt{(d_{AB})} r_{cov,B}/CN_B}{\|r_{cov,B}/x_A - x_B d_{AB}\|}$<br>$d_2 = \frac{V_{\text{cell}}}{\sum V_{\text{atom}}} \frac{\chi_A}{\exp(CN_A)(r_{cov,B}/d_{AB} - x_B + x_A)}$ |

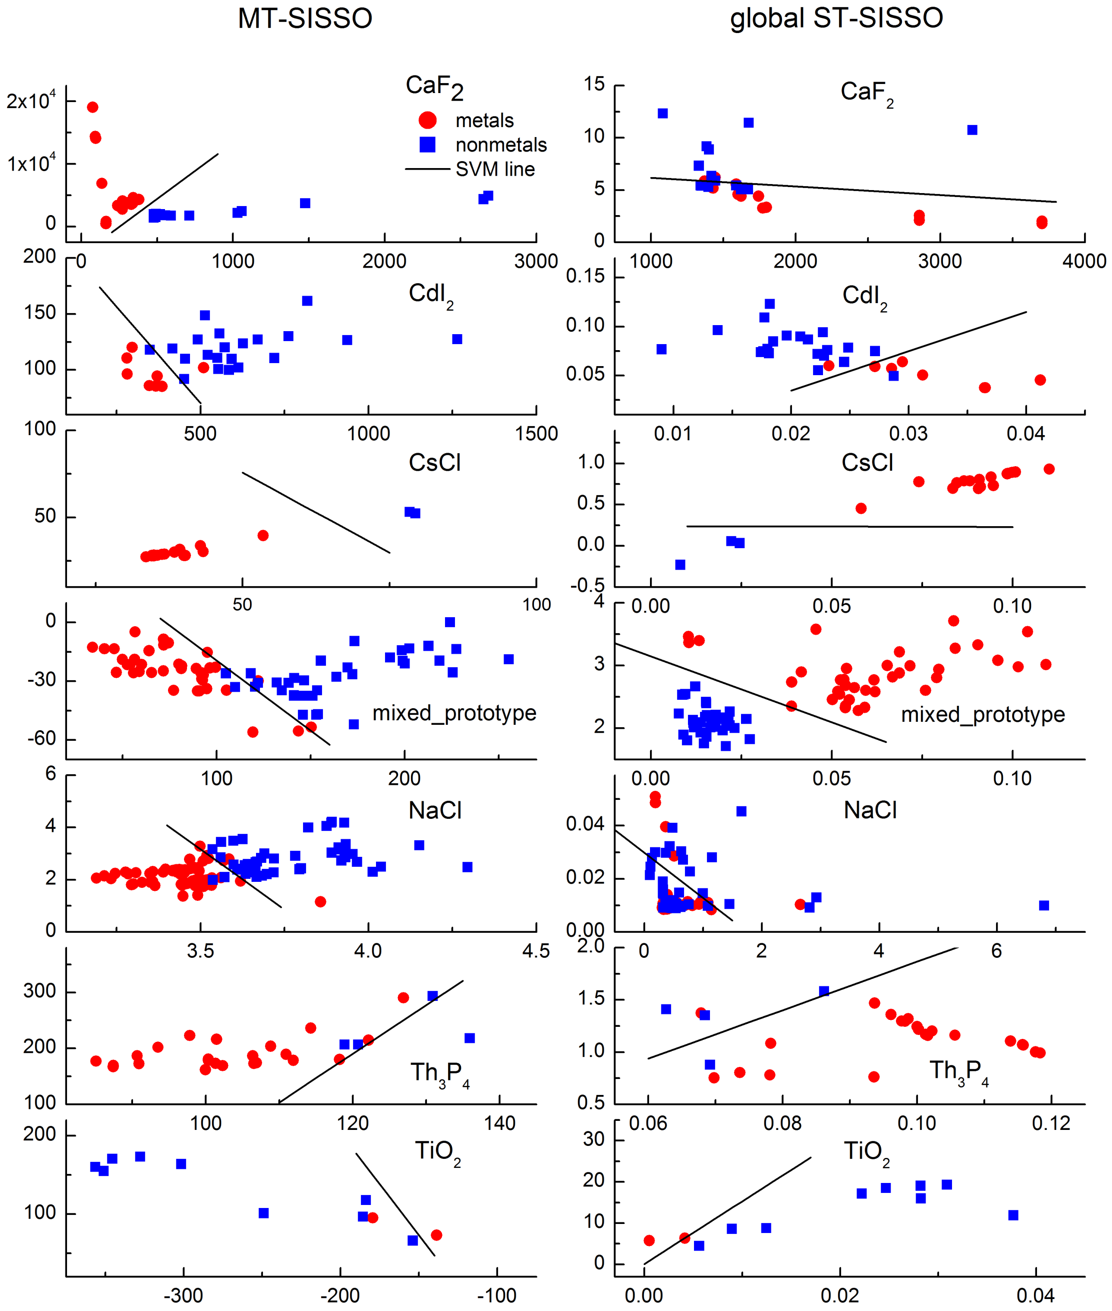


FIG. 1: Leave-prototype-out generalization test for MT-SISSO and global ST-SISSO. Both MT-SISSO and ST-SISSO descriptors are trained on all prototypes except the left out one, and they are shown in Table II. The support-vector-machine (SVM) line is trained on the data of the left out prototype, with the descriptor fixed. For MT-SISSO, the number of misclassified data of the test prototypes are: 0 (CsCl prototype), 1 ($TiO_2$), 2 ($CdI_2$), 3 ($Th_3P_4$), 0 ($CaF_2$), 5 (mixed-prototype: 2 NiAs, 1 $ThH_2$, 2 ZnS), and 6 (NaCl). For global ST-SISSO, the number of misclassified data of the test prototypes are: 0 (CsCl), 1 ($TiO_2$), 2 ($CdI_2$), 2 ($Th_3P_4$), 7 ($CaF_2$), 0 (mixed-prototype), 36 (NaCl).
